# Supplementary material for: Quantum disordered ground state in the spin-orbit coupled Jeff = 1/2 distorted honeycomb magnet BiYbGeO5
Source: arXiv:2305.10221 source file (2023-05-17)
Supplement: Supplementary file 1 [file SM.pdf]

# Quantum disordered ground state in the spin-orbit coupled $J_{\text{eff}} = \frac{1}{2}$ distorted honeycomb magnet $BiYbGeO_5$

S. Mohanty,[1] S. S. Islam,[1] N. Winterhalter-Stocker,[2] A. Jesche,[2] G. Simutis,[3] Ch. Wang,[4] Z. Guguchia,[4] J. Sichelschmidt,[5] M. Baenitz,[5] A. A. Tsirlin,[6] P. Gegenwart,[2] and R. Nath[1,*]

[1] *School of Physics, Indian Institute of Science Education and Research Thiruvananthapuram-695551, India*
[2] *Center for Electronic Correlations and Magnetisim, University of Augsburg, 86159 Augsburg, Germany*
[3] *Laboratory for Neutron and Muon Instrumentation, Paul Scherrer Institut, CH-5232 Villigen PSI, Switzerland*
[4] *Laboratory for Muon Spin Spectroscopy, Paul Scherrer Institut, Villigen PSI, Switzerland*
[5] *Max Planck Institute for Chemical Physics of Solids, Nothnitzer Str: 40, 01187 Dresden, Germany*
[6] *Felix Bloch Institute for Solid-State Physics, Leipzig University, 04103 Leipzig, Germany*

(Dated: May 17, 2023)

## EXPERIMENTAL DETAILS

Polycrystalline samples of Bi$Re$GeO$_5$ ($Re$ = Yb, Y) were synthesized using the conventional solid-state reaction technique. $Bi_2O_3$ (99.99 %, trace metals basis, Sigma Aldrich), $GeO_2$(99.99 %, trace metals basis, Sigma Aldrich), and $Re_2O_3$ (99.99 %, trace metals basis, Sigma Aldrich) were used as starting precursors. The stoichiometric mixtures of the starting materials were thoroughly ground, pressed into pellets, heated in a platinum crucible at 950°C for two days in air, and then quenched. Excess 4 % $Bi_2O_3$ was used as the starating material to get the pure phase of Bi$Re$GeO$_5$. The phase purity of the sample was confirmed by the powder x-ray diffraction (XRD) measurement using the PANalytical x-ray diffractometer (Cu $K_\alpha$ radiation, $\lambda_{\text{av}} \simeq 1.5418$ Å).

Magnetization ($M$) measurements were performed as a function of temperature ($T$) and applied field ($H$) using a superconducting quantum interference device (SQUID) (MPMS-3, Quantum Design). Measurements down to 0.4 K were carried out using a $^3$He (iHelium3, Quantum Design Japan) attachment to the MPMS.

Heat capacity [$C_{\text{p}}(T)$] for $T > 1.8$ K was measured on a small piece of sintered pellet using the relaxation technique in the physical property measurement system (PPMS, Quantum Design). For the measurements in the milli-Kelvin range, we have used a pellet of the mixture (1:1 ratio) of $BiYbGeO_5$ and fine Ag powder of total mass of 9.41 mg and the measurements were carried out using the thermal relaxation method with a home-built setup installed in a dilution refrigerator. Here, the fine Ag powder is crucial for realizing a good thermal contact at low temperatures. The contribution of the Ag-powder to the heat capacity was determined from a polynomic function with the coefficients from Ref. [S1] and subtracted from total measured heat capacity. In a magnetic insulator, the heat capacity contains contributions from the phonon excitations ($C_{\text{ph}}$), the magnetic lattice ($C_{\text{mag}}$), and the nuclear quadrupolar moment ($C_{\text{n}}$). At high temperatures, $C_{\text{p}}$ is entirely dominated by $C_{\text{ph}}$, while at low temperatures, it has dominant contributions from $C_{\text{mag}}$ and $C_{\text{n}}$. Magnetic heat capacity ($C_{\text{mag}}$) is estimated by subtracting $C_{\text{ph}}$ and $C_{\text{n}}$ from the total measured heat capacity (*i.e.* $C_{\text{mag}} = C_{\text{p}}$ - $C_{\text{ph}}$ - $C_{\text{n}}$).

We investigated the Electron Spin Resonance (ESR) on polycrystalline $BiYbGeO_5$ sample using a standard continuous-wave ESR setup at X-band frequency (9.4 GHz). The temperature was varied between 3 and 295 K with a He-flow cryostat. ESR can be detected by the absorbed power $P$ of a transversal magnetic microwave field as a function of a static, external magnetic field $\mu_0 H$. To improve the signal-to-noise ratio, we used a lock-in technique by modulating the static field, which yields the derivative of the resonance signal $dP/dH$. The measured ESR spectra were fitted with a Lorentzian function including the influence of the counter-rotating component of the linearly polarized microwave field [S2]. From the fit we obtained the linewidth $\Delta H$ and the resonance field $H_{\text{res}}$ which determines the ESR $g$-factor, $g = h\nu/\mu_B H_{\text{res}}$. The ESR intensity $I_{ESR}$ is a measure of the local static susceptibility of the probed ESR spin, i.e. in our case the local susceptibility of the $Yb^{3+}$ spins. We calculated $I_{\text{ESR}} \approx Amp \cdot \Delta H^2$ which approximates the integrated ESR absorption.

Muon spin relaxation ($\mu^+$SR) measurements were carried out on the powder sample at the Swiss Muon Source (S$\mu$S), Paul Scherrer Institute, Switzerland with the help of two spectrometers. The high temperature measurements (1.5 K - 50 K) were performed using low-background high-throughput instrument, General Purpose Spectrometer (GPS) in zero-field as well as in longitudinal fields [S3]. The low temperature measurements in both zero and transverse fields were performed using the standard settings of the HAL spectrometer which allowed reaching temperatures as low as 12 mK. For the measurement purpose, powder sample was packed in silver(Ag) foil envelopes, attached to a silver

plate and mounted on the cold finger of the dilution refrigerator. Ag was used because of its small nuclear magnetic moment which minimizes the background depolarization of the muon spin ensemble.

## X-RAY DIFFRACTION

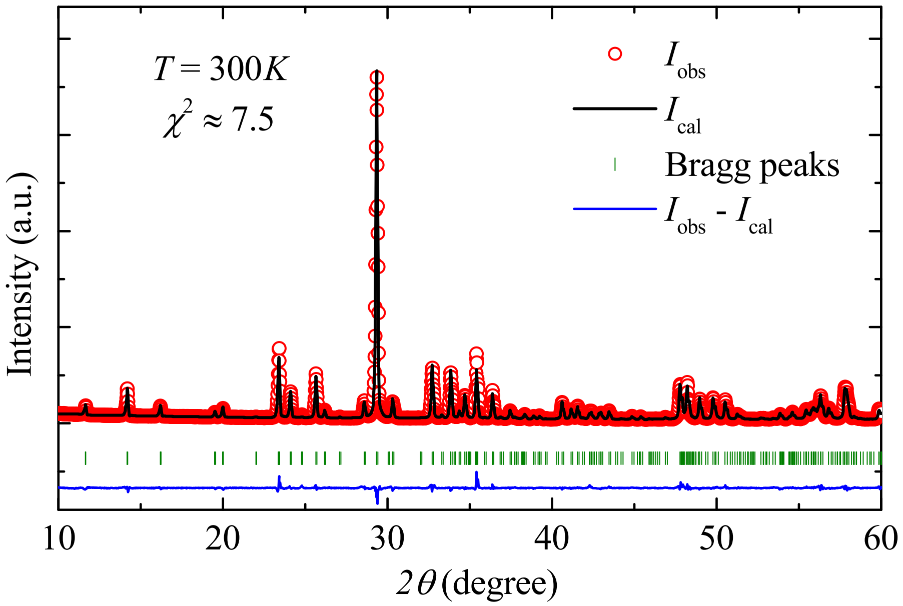


FIG. S1. Powder XRD pattern (open circles) at $T = 300$ K. The black solid line represents the Rietveld fit of the data. Expected Bragg positions are indicated by green vertical bars and the solid blue line at the bottom denotes the difference between experimental and calculated intensities. The goodness-of-fit is achieved to be $\chi^2 \simeq 7.5$.

TABLE S1. Listed are the Wyckoff positions and the refined atomic coordinates ($x$, $y$, and $z$) for each atom at room temperature.

| Atom | Site | $x$ | $y$ | $z$ | Occupancy |
|---|---|---|---|---|---|
| Bi1 | 8c | 0.9560(3) | 0.2382(1) | 0.1458(1) | 1 |
| Yb1 | 8c | 0.0119(5) | 0.0514(1) | 0.3600(2) | 1 |
| Ge1 | 8c | 0.0085(1) | 0.4035(2) | 0.4021(3) | 1 |
| O1 | 8c | 0.0385(4) | 0.2755(1) | 0.3534(1) | 1 |
| O2 | 8c | 0.3034(4) | 0.4278(1) | 0.4333(2) | 1 |
| O3 | 8c | 0.3154(3) | 0.0922(2) | 0.4743(1) | 1 |
| O4 | 8c | 0.2574(6) | 0.1718(1) | 0.2605(4) | 1 |
| O5 | 8c | 0.3408(3) | 0.4699(1) | 0.1998(1) | 1 |

$BiYbGeO_5$ belongs to a family having general formula Bi*Re*$GeO_5$ ($Re$ = Rare-earth) with the orthorhombic crystal system of space group *Pbca* (No. 61) [S4]. Each Yb atom is coordinated to seven oxygen atoms forming $YbO_7$ polyhedra which constitutes $YbO_6$ trigonal prisim capped by one oxygen atom on the face simialr to a monocapped trigonal prisim. The $YbO_7$ polyherda are joined through the O4-O5 edge in the $a$-direction and through O2-O2 in the $c$-direction, forming buckled honeycomb layers in the $ac$-plane.

In order to confirm the phase purity and crystal structure of the sample, powder XRD was collected at room temperature. Rietveld refinement of the XRD data was carried out using `FullProf` software package, that confirms the formation of pure phase shown in Fig. S1. All peaks in the XRD data could be appropriately indexed by the space group *Pbca* (No. 61) and the obtained lattice parameters at room temperature are $a = 5.2948(1)$ Å, $b = 15.2015(2)$ Å, $c = 10.9437(2)$ Å, and $V_{\rm cell} \simeq 880.85(3)$, which are fairly comparable with the previous report [S4]. The atomic coordinates of different atoms after the refinement are tabulated in Table S1.

## MAGNETIZATION

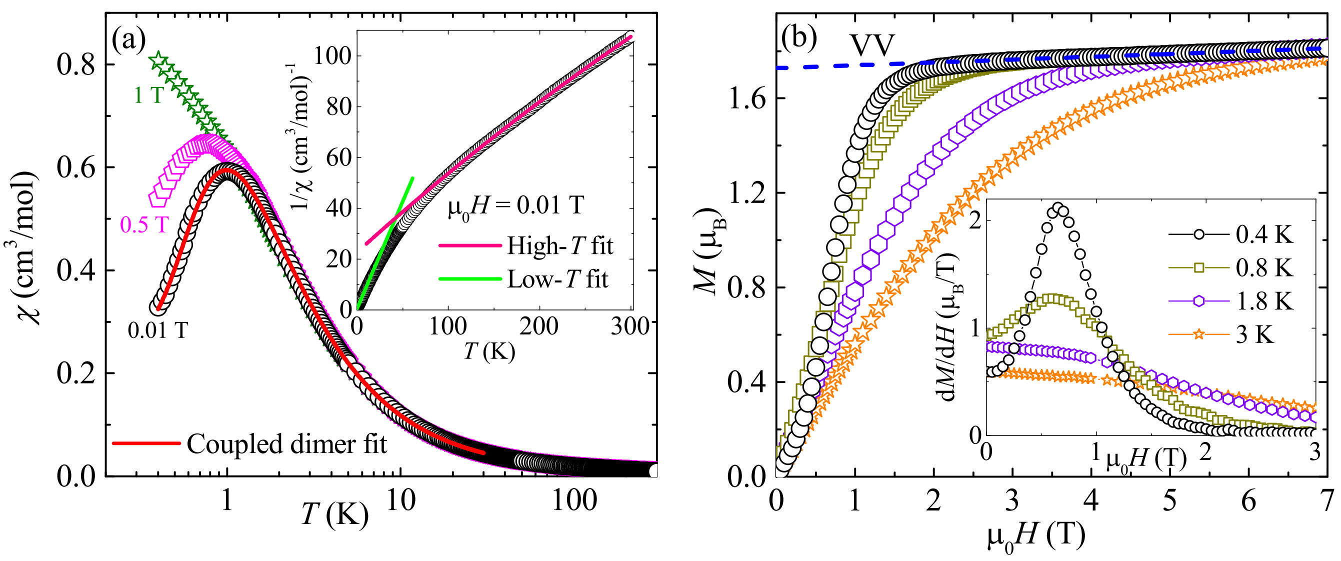


FIG. S2. (a) $\chi(T)$ of $BiYbGeO_5$ measured at different magnetic fields. The solid line represents the fit of the 0.01 T data by the interacting dimer model. Inset: CW fits to the $1/\chi$ data at 0.01 T in the low-temperature and high-temperature regimes. (b) $M$ vs $H$ measured at different temperatures. The horizontal dashed line marks the Van-Vleck contribution. Inset: $dM/dH$ vs $H$ to highlight the field-induced features.

Magnetic susceptibility ($\chi$) as a function of $T$ in various applied fields is depicted in Fig. S2(a). The rapid decrease of $\chi(T)$ in a low field of 0.01 T below the broad maximum is indicative of a singlet ground state. With increasing field the broad maxima shifts towards low temperatures reflecting the closing of spin-gap. The inverse susceptibility ($1/\chi$) for $H = 0.01$ T [inset of Fig. S2(a)] shows two linear regimes at high and low temperatures with a slope change at around 50 K. This possibly reflects a spin cross-over from high-spin ($J = 7/2$) to low-spin ($J_{\rm eff} = 1/2$) state. The fit above 150 K by $\chi_0 + \frac{C}{T-\theta_{\rm CW}}$ (where $\chi_0$ is the temperature independent susceptibility and the second term is the CW law) yields $\chi_0 \simeq 1.5\times10^{-3}$ cm$^3$/mol, a high-$T$ effective moment $\mu_{\rm eff}^{\rm HT}$ [$= \sqrt{3k_{\rm B}C/N_{\rm A}}$, where $C$, $k_{\rm B}$, and $N_{\rm A}$ are the Curie constant, Boltzmann constant, and Avogadro's number, respectively] $\simeq 4.78\ \mu_{\rm B}$, and the high-$T$ CW temperature $\theta_{\rm CW}^{\rm HT} \simeq -67.2$ K. This value of $\mu_{\rm eff}^{\rm HT}$ is in good agreement with the expected value, $\mu_{\rm eff} = g\sqrt{J(J+1)} \simeq 4.54\ \mu_{\rm B}$ for $Yb^{3+}$ ($J = 7/2$, $g = 8/7$) in the $^4f_{13}$ configuration.

In the main text, we show that the model of anisotropic spin dimers ($J_{\rm XY} \neq J_{\rm Z}$) captures all thermodynamic properties of $BiYbGeO_5$. Interestingly, a good fit of the magnetic susceptibility is also possible with the model of Heisenberg spin dimers if a weak interdimer interaction is included. Experimental $\chi(T)$ data were fitted [see Fig. S2(a)] by the following expression,

$$\chi(T) = \chi_0 + \frac{C_{\rm imp}}{T} + \frac{N_{\rm A}g^2\mu_{\rm B}^2}{k_{\rm B}T[3+\exp(J_0/k_{\rm B}T)+zJ'/k_{\rm B}T]}, \quad \text{(S1)}$$

where $C_{\rm imp}$ is the Curie constant corresponding to impurity spins. The third term is the susceptibility of a Heisenberg spin dimer with the mean-field correction for the interdimer couplings $J'$ [S5], whereas $z = 4$ is the number of the neighboring dimers. Equation (S1) fits the $\chi(T)$ data very well in the $T$-range 0.4 K $\leq T \leq$ 30 K yielding $\chi_0 \simeq 5\times10^{-3}$ cm$^3$/mol, $C_{\rm imp} \simeq 4.9\times10^{-2}$ cm$^3$K/mol, $g \simeq 3.5$, $J_0/k_{\rm B} \simeq 1.7$ K, and $J'/k_{\rm B} \simeq 0.06$ K. From the value of $C_{\rm imp}$, the concentration of impurity spins is found to be nearly $\sim 4.2$ %, assuming the impurity spins $S = 1/2$ and $g = 3.5$.

Figure S2(b) presents the magnetic isotherms ($M$ vs $H$) measured at various temperatures in the low-$T$ regime. The $dM/dH$ vs $H$ plot in the inset of Fig. S2(b) clearly features a rounded maximum at $H_{\rm C} \sim 0.65$ T. This rounded maximum diminishes gradually with increasing temperature, as expected.

Figure S3 presents the measurement results in zero field cooled (ZFC) and field cooled (FC) protocols that depict no bifurcation, suggesting the absence of spin freezing or spin-glass transition down to $T = 2$ K.

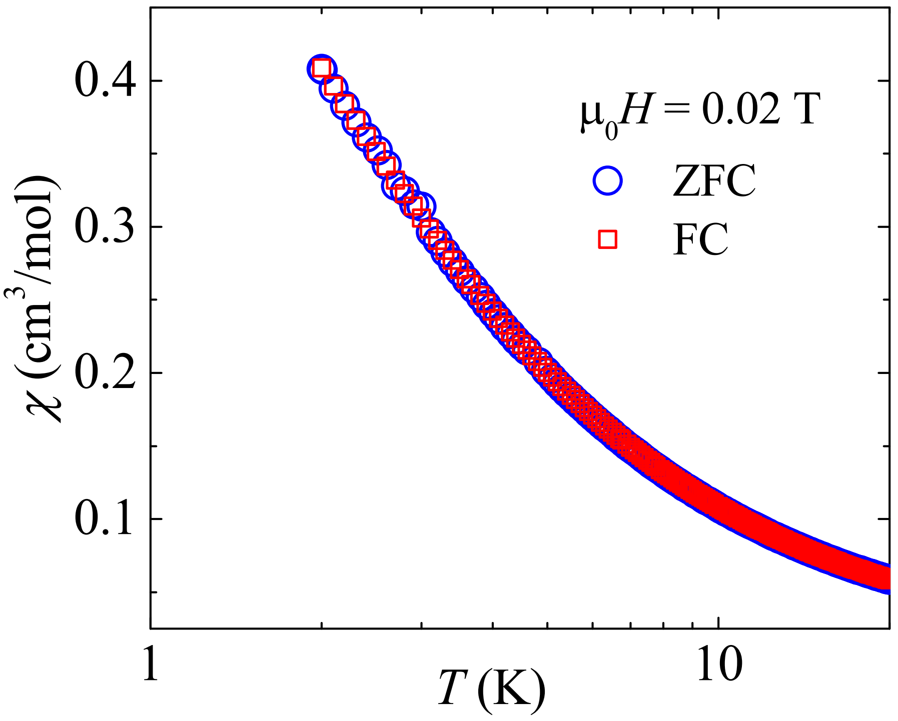


FIG. S3. Absence of bifurcation pictured in the $\chi$ vs $T$ plot between ZFC and FC data at $H = 200$ Oe.

## HEAT CAPACITY

Heat Capacity ($C_\mathrm{p}$) vs applied field ($H$) measured at two lowest temperatures $T = 0.08$ K and $T = 0.100$ K is shown in Fig. S4.

## ELECTRON SPIN RESONANCE

Electron spin resonance (ESR) spectra for two typical temperature regimes are shown in Fig. S5(a). Red solid lines depict symmetrical Lorentzian shape with corresponding $g$-value of $g = 3.2(5)$ at $T = 15$ K. The ESR intensity $I_\mathrm{ESR}$ which is a measure of bulk magnetic susceptibility follows a Curie-Weiss behaviour in the low temperature regime. As shown in Fig. S5(b), $I_\mathrm{ESR}^{-1}$ as a function of $T$ shows two linear regimes at high and low temperatures. The Curie-Weiss fit to the low temperature (3 - 20 K) data yields $\theta_\mathrm{CW} \simeq -0.66$ K.

The temperature dependence of the ESR linewidth ($\Delta H$) is shown in Fig. S5(c). For $T \geq 60$ K, the ESR linewidth broadens according to $\Delta H \propto 1/\exp(\Delta/T) - 1$. This behavior indicates a spin-lattice relaxation dominated by an Orbach process. Via spin-orbit coupling this process involves a phonon absorption to and emission from a crystalline-electric field split electronic energy level $\Delta$ above the ground state [S6]. We obtained $\Delta = (600 \pm 100)$ K. Towards low temperatures, no broadening is observed and the linewidth approaches a constant value of 150 mT. A broadening would have been expected from the growing influence of $Yb^{3+}$ spin correlations at low temperatures.

## MUON SPIN RELAXATION

### Zero field measurement

Temperature dependent zero-field muon asymmetry curves are displayed in Fig S6. In a magnetic ordered state, muon decay asymmetry exhibits oscillating signal and a non-oscillating undamped 1/3 tail in the case of polycrystalline samples. Neither of the two features are present in the data, ruling out a uniform magnetic ordering down to 12 mK.

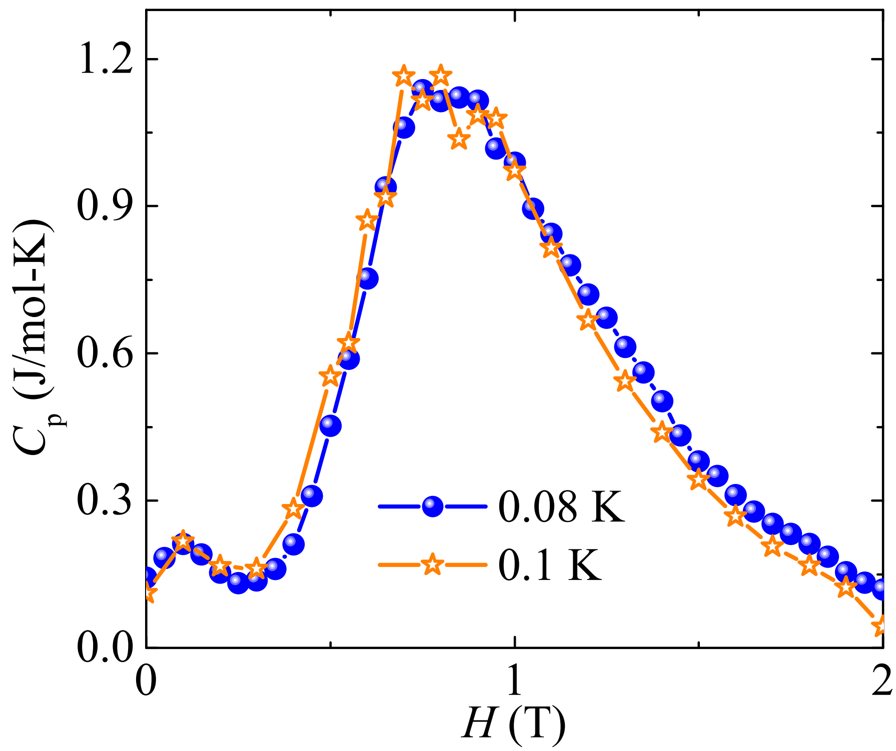


FIG. S4. $C_p$ vs $H$ measured to $T = 0.08$ K and $T = 0.100$ K.

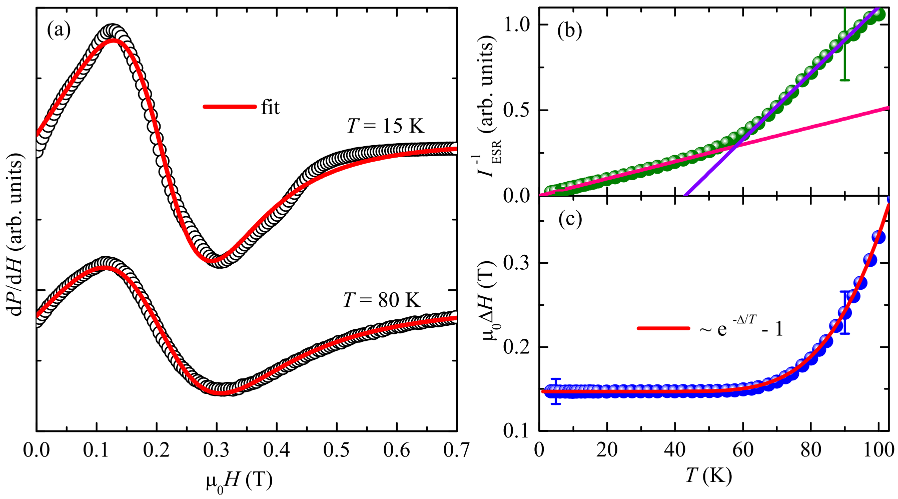


FIG. S5. (a) Magnified ESR spectra of $BiYbGeO_5$ at two temperatures. The red solid lines depict Lorentzian line shape. (b) Temperature dependent reciprocal ESR intensity $I_{\mathrm{ESR}}^{-1}$ with solid lines guiding the linear behavior. (c) ESR linewidth $\Delta H$ vs $T$ where the solid line refers at higher temperatures to a relaxation mechanism via the first excited crystalline electric field level of $Yb^{3+}$ with $\Delta = (600 \pm 100)$ K.

The asymmetry curves are fitted by a stretched exponential function:

$$A(t) = A(0)e^{-(\lambda t)^{\beta}}. \tag{S2}$$

To account for the shape of the muon depolarization curve, a stretching exponent $\beta$ is introduced, which suggests that there is a distribution of the relaxation rates. The stretching exponent is found to be constant to 0.73 for all the temperatures. The obtained depolarization rate ($\lambda$) is found to be approximately constant at high temperatures and exhibits a drop as the sample is cooled down below around 10 K (inset of Fig S6). At temperatures below around

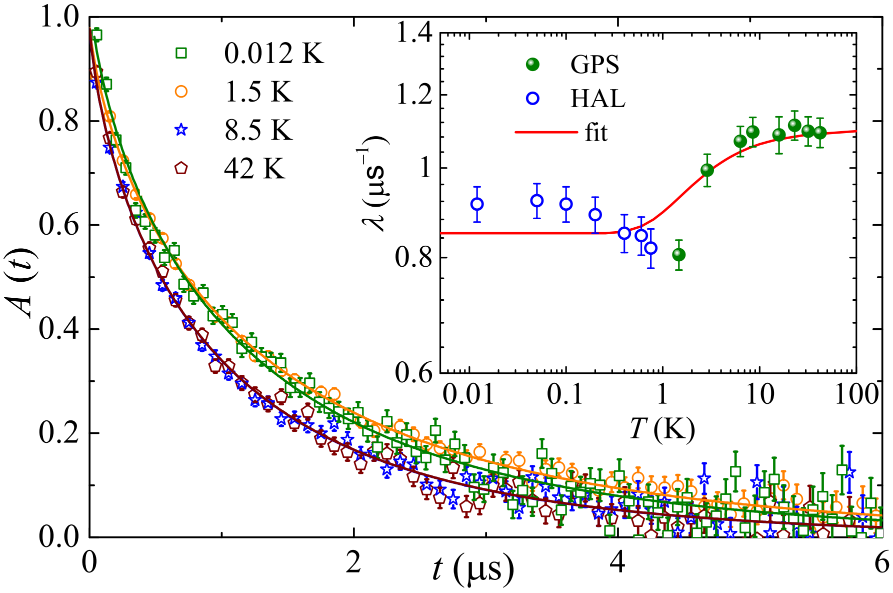


FIG. S6. Muon decay asymmetry as a function of time in zero-field for few representative temperatures. Solid lines are the fits using Eq. (S2). Inset: Muon depolarization rate ($\lambda$) vs $T$ in zero-field measured in both GPS and HAL spectrometers. The solid line represents an exponential fit.

1 K, $\lambda$ stays at a smaller constant value. This behavior is consistent with an exponential decay with a spin-gap of $\Delta/k_{\rm B} \simeq 1.7$ K.

**Transverse field measurement at HAL ($T = 12$ mK and 300 mK)**

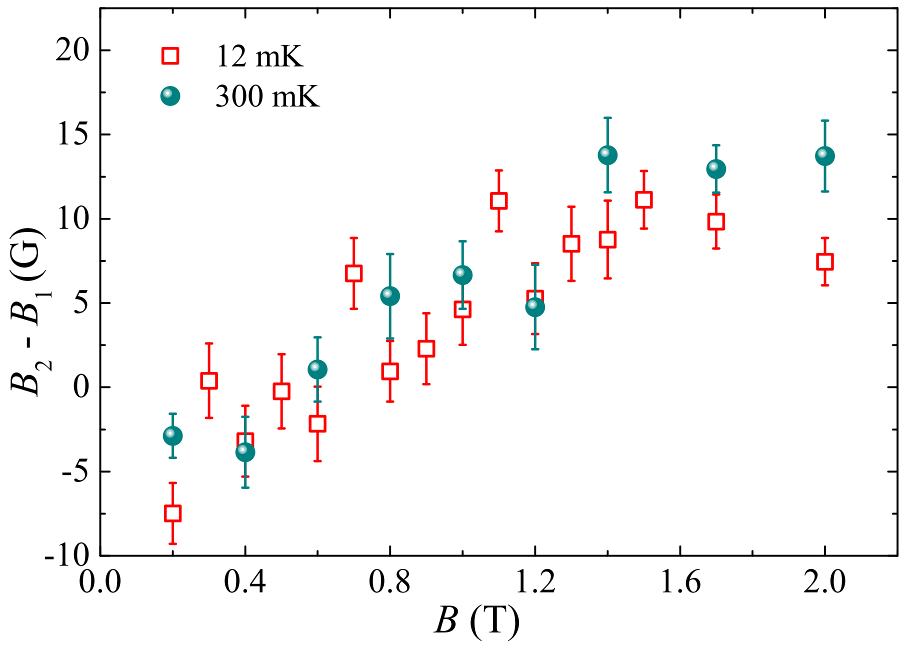


FIG. S7. Difference between the internal fields felt by the muons as a function of applied magnetic field (transverse).

To study a potential Bose-Einstein condensation of triplons, we have then performed field scans up to 2 T in transverse fields at $T = 300$ mK and 12 mK. The muon decay asymmetry changes very little with the application of

such fields, ruling out a field induced LRO. The response is best described by two components. One is likely arising from parts of the sample that don't feel additional magnetic field as well as a contribution from the sample holder and has a slow depolarization rate (about 0.4 $\mu$s and independent of temperature and field). The second component is from muons implanted in the positions of the sample where they feel a magnetic field with a broader distribution, leading to a faster depolarisation rate (about 6 $\mu$s and also independent of temperature and field). The only quantity that shows field dependence is the difference between the peak positions of the two components and is plotted in Fig S7. There appears to be no temperature dependence and the behavior as a function of field is somewhat similar to that observed for magnetization.

### Longitudinal field measurement at GPS ($T = 1.5$ K)

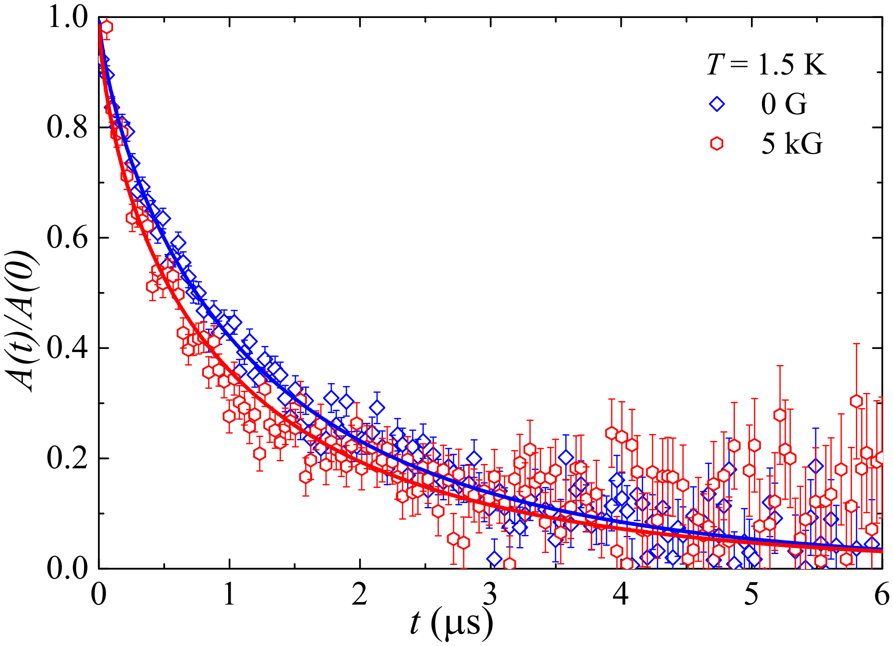


FIG. S8. Depolarization rate as a function of time for two different longitudinal fields at $T = 1.5$ K.

Very surprising effect has been observed while applying longitudinal field to the system. Usually, the depolarization rate is suppressed upon application of the longitudinal field, however, here we find an increase of depolarization rate at low temperatures as seen in Fig. S8. At the moment this is not understood.


[S1] D. L. Martin, Specific heat of copper, silver, and gold below 30°k, Phys. Rev. B **8**, 5357 (1973).

[S2] D. Rauch, M. Kraken, F. J. Litterst, S. Süllow, H. Luetkens, M. Brando, T. Förster, J. Sichelschmidt, A. Neubauer, C. Pfleiderer, W. J. Duncan, and F. M. Grosche, Spectroscopic study of metallic magnetism in single-crystalline $Nb_{1-y}Fe_{2+y}$, Phys. Rev. B **91**, 174404 (2015).

[S3] A. Amato, H. Luetkens, K. Sedlak, A. Stoykov, R. Scheuermann, M. Elender, A. Raselli, and D. Graf, The new versatile general purpose surface-muon instrument (GPS) based on silicon photomultipliers for $\mu$SR measurements on a continuous-wave beam, Rev. Sci. Instrum. **88**, 093301 (2017).

[S4] C. Cascales, J. A. Campa, E. G. Puebla, M. A. Monge, C. R. Valero, and I. Rasines, New rare-earth (Y, Yb) bismuth(iii) germanates. an initial study of a promising series, J. Mater. Chem. **12**, 3626 (2002).

[S5] A. A. Aczel, Y. Kohama, C. Marcenat, F. Weickert, M. Jaime, O. E. Ayala-Valenzuela, R. D. McDonald, S. D. Selesnic, H. A. Dabkowska, and G. M. Luke, Field-induced Bose-Einstein condensation of triplons up to 8 K in $Sr_3Cr_2O_8$, Phys. Rev. Lett. **103**, 207203 (2009).

[S6] R. Orbach and B. Bleaney, Spin-lattice relaxation in rare-earth salts, Proc. Math. Phys. Eng. Sci. **264**, 458 (1961)
